# Supplementary material for: Unsupervised Word Segmentation from Discrete Speech Units in Low-Resource Settings
Source: arXiv:2106.04298 source file (2022-05-18)
Supplement: Supplementary file 1 [file 6_appendix.tex]

\clearpage
\section{Appendix}\label{sec:appendix}
\subsection{Training Parameters}\label{sec:appendix1}
\paragraph{VQ-VAE.} We used the implementation provided at:  \url{github.com/BUTSpeechFIT/vq-aud}. 
%The encoder is composed of 4 BLSTM layers each with output dimension 128 followed by a 16-dimensional and a feed-forward decoder with one hidden layer. The number of discovered units  (quantization centroids) is set to 50. This setting is unusually low but helps to reduce the length of the output sequence. We set $k_1 = 2$ and $k_2 = 4$. We train with Adam with an initial learning rate of $2\times10^{-3}$ which is halved whenever the loss stagnates for two training epochs. The model is trained on the Mboshi and Russian datasets presented in the paper.

\paragraph{Bayesian AUD models.} We used the implementation provided at: \url{https://github.com/beer-asr/beer/tree/master/recipes/hshmm}. %For all the Bayesian AUD models, we use 4 Gaussians per HMM state and we set the truncation parameter of the Dirichlet process to 100. We use 100-dimensional unit embeddings of the SHMM and the H-SHMM. Furthermore, we use 6-dimensional language embeddings for the H-SHMM. The transferred SHMM and H-SHMM subspaces are estimated with French, German, Spanish, Polish from the Globalphone corpus~\cite{schultz2013globalphone}, as well as Amharic~\cite{Abate2005amharic}, Swahili~\cite{gelas2012swahili} and Wolof~\cite{gauthier2016wolof} from the ALFFA project~\cite{besacier2015speech}. 

\paragraph{UWS models.} The Bayesian UWS models (\textit{dpseg}\footnote{Available at \url{http://homepages.inf.ed.ac.uk/sgwater/resources.html}}) use the settings from \citet{godard2016preliminary}, and the unigram model. We train three models for each representation, averaging the obtained results. The neural UWS models use the parameters from \citet{Boito2019} and the implementation described in \citet{Godard2018}. We train five models for each representation, averaging the soft-alignment probability matrices before performing segmentation. UWS boundary evaluation uses the Zero Resource Challenge implementation available at: \url{http://zerospeech.com/2017}.

%\clearpage
\subsection{Table and Figures}
